# Supplementary material for: Anomalous spin Hall angle of a metallic ferromagnet determined by a multiterminal spin injection/detection device
Source: arXiv:1905.00663 ancillary file (2019-05-02)
Supplement: Supplementary file 1 [file SI_Magnon_transport_CoFe.pdf]

# Supplementary Information: Anomalous spin Hall angle in a metallic ferromagnet determined by a multiterminal spin injection/detection device

T. Wimmer,[1,2,*] B. Coester,[3] S. Geprägs,[1] R. Gross,[1,2,4,5]
S. T. B. Goennenwein,[6] H. Huebl,[1,2,4,5] and M. Althammer[1,2,†]

[1] *Walther-Meißner-Institut, Bayerische Akademie der Wissenschaften, 85748 Garching, Germany*

[2] *Physik-Department, Technische Universität München, 85748 Garching, Germany*

[3] *School of Physical and Mathematical Sciences, Nanyang Technological University, 21 Nanyang Link, Singapore 637371, Singapore*

[4] *Nanosystems Initiative Munich (NIM), Schellingstraße 4, 80799 München, Germany*

[5] *Munich Center for Quantum Science and Technology (MCQST), Schellingstr. 4, D-80799 München, Germany*

[6] *Institut für Festkörper- und Materialphysik and Würzburg-Dresden Cluster of Excellence ct.qmat, Technische Universität Dresden, 01062 Dresden, Germany*

(Dated: April 23, 2019)

* tobias.wimmer@wmi.badw.de

† matthias.althammer@wmi.badw.de

## A. Determination of the YIG/Pt spin conductance via spin Hall magnetoresistance measurements

The spin conductance $g_{\mathrm{Pt}}$ of the YIG/Pt interfaces can be deduced from spin Hall magnetoresistance (SMR) measurements on the Pt electrodes. The magnitude of the SMR is given by the relative resistivity change $\Delta R_{\mathrm{long}}/R_{\mathrm{long}}$ in the Pt electrode measured between the in-plane YIG magnetization pointing parallel and perpendicular to the current direction. The theoretical equation for the SMR magnitude reads [S1]

$$\frac{\Delta R_{\mathrm{long}}}{R_{\mathrm{long}}} = \frac{{\Theta_{\mathrm{SH}}^{\mathrm{Pt}}}^2 \lambda_{\mathrm{Pt}}}{t_{\mathrm{Pt}}} \frac{2\lambda_{\mathrm{Pt}} g_{\mathrm{Pt}}^{\uparrow\downarrow} \tanh^2(\frac{t_{\mathrm{Pt}}}{2\lambda_{\mathrm{Pt}}})}{\sigma_{\mathrm{Pt2}} + 2\lambda_{\mathrm{Pt}} g_{\mathrm{Pt}}^{\uparrow\downarrow} \coth(\frac{t_{\mathrm{Pt}}}{\lambda_{\mathrm{Pt}}})}, \tag{S1}$$

where $g_{\mathrm{Pt}}^{\uparrow\downarrow}$ is the spin mixing conductance [S2] of the YIG/Pt interfaces and $\sigma_{\mathrm{Pt2}}$ is the conductivity of the Pt2 electrode. We measured the longitudinal resistance $R_{\mathrm{long}}$ at the Pt2 electrode as a function of the magnetic field orientation $\varphi$ for various magnetic fields, as shown in Fig. S1 (a). The resistance change is determined by fitting a $\Delta R_{\mathrm{long}} \sin^2(\varphi)$ function to the magnetization orientation dependent data (under the assumption that the magnetization in the YIG is always aligned parallel to the external magnetic field), extracting $\Delta R_{\mathrm{long}}$ and normalizing it to the high resistance value $R_{\mathrm{long}}$. The resulting SMR magnitude is shown as a function of the external magnetic field in Fig. S1 (b). As expected from Theory [S1], we do not see any significant field dependence of the SMR. In order to obtain a representative value, we calculate an average over the whole field range measured and find $\Delta R_{\mathrm{long}}/R_{\mathrm{long}} = 7.38 \times 10^{-5}$. Hence, we can calculate the spin mixing conductance from Eq. (S1). Using the values listed in Tab. S1, we find $g_{\mathrm{Pt}}^{\uparrow\downarrow} = 2.68 \times 10^{13}\,\mathrm{S\,m^{-1}}$. According to Ref. S3, the spin conductance $g_{\mathrm{Pt}}$ relates to the spin mixing conductance as $g_{\mathrm{Pt}} = 0.06 g_{\mathrm{Pt}}^{\uparrow\downarrow} = 1.61 \times 10^{12}\,\mathrm{S\,m^{-1}}$ at room temperature. This value is then used throughout the calculations shown in the main text.

## B. Magnon diffusion length

The spin-resistor model that we applied to our magnon transport structure in the main text is only valid if the magnon diffusion length of our YIG film is larger than the distances between the respective electrodes considered. We thus measured the magnon diffusion length $\lambda_{\mathrm{m}}$ of a comparable $1\,\mu\mathrm{m}$ thick YIG film from the same wafer as the one studied in the main text. For this purpose, we structured simple two-electrode devices consisting of Pt

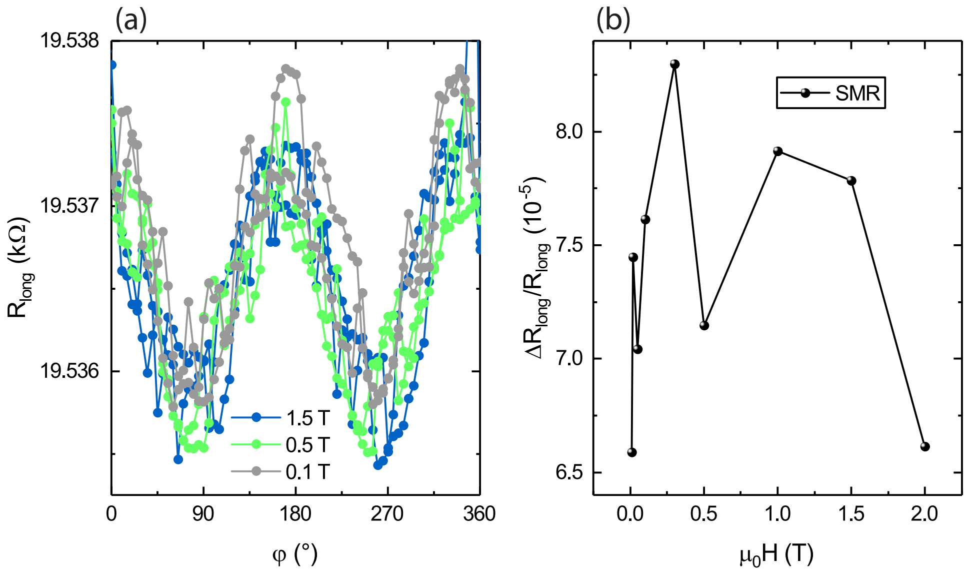


FIG. S1. (a) Longitudinal resistance $R_{\text{long}}$ measured on the Pt2 electrode as a function of the magnetic field orientation $\varphi$ for different magnetic field magnitudes. (b) SMR magnitude $\Delta R_{\text{long}}/R_{\text{long}}$ as a function of magnetic field.

| | Symbol | Value | Unit |
|---|---|---|---|
| Pt strip thickness | $t_{\text{Pt}}$ | 7 | nm |
| CoFe strip thickness | $t_{\text{CoFe}}$ | 7 | nm |
| Pt & CoFe strip widths | $w$ | 500 | nm |
| Pt spin diffusion length [S4] | $\lambda_{\text{Pt}}$ | 1.5 | nm |
| Pt spin Hall angle [S4] | $\theta_{\text{SH}}^{\text{Pt}}$ | 0.11 | |
| Pt2 conductivity | $\sigma_{\text{Pt2}}$ | $2.64 \times 10^6$ | $1/\Omega\text{m}$ |
| CoFe conductivity | $\sigma_{\text{CoFe}}$ | $1.50 \times 10^6$ | $1/\Omega\text{m}$ |
| YIG thickness | $t_{\text{YIG}}$ | 1 | µm |

TABLE S1. Values used for the calculations discussed in the main text, as well as for Eq. (S1).

strips, with a thickness of 7 nm on the YIG film with various separation distances $d$ (here $d$ denotes the edge-to-edge distance between the electrodes). In Fig. S2 (a) the distance dependence of the magnon transport signal $V_{\text{det}}$ is plotted for different external magnetic fields. As indicated by the green and gray areas in the plot, we observe two different

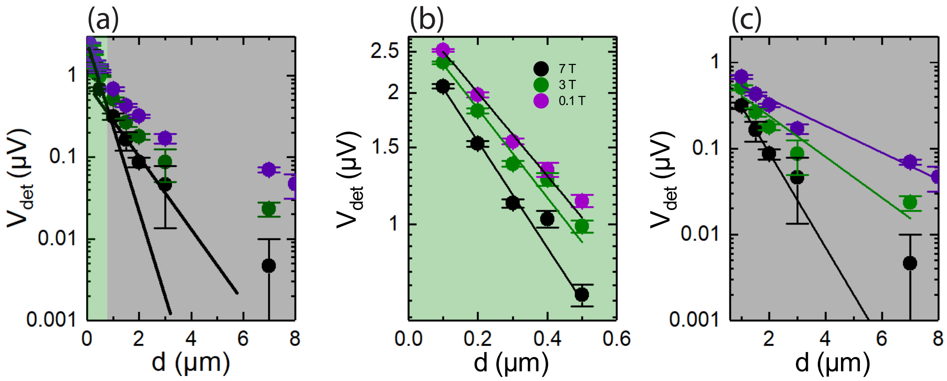


FIG. S2. (a) Distance dependence of the magnon transport signal $V_{\mathrm{det}}$ plotted on a logarithmic scale. The data is measured for a comparable 1 μm thick YIG film from the same wafer as the one studied in the main text. The straight lines indicate the different behaviours on different length scales. Short (long) distances are indicated in green (grey) areas. Panels (b) and (c) show an enlarged view of the short and long distance regimes with exponential fits, respectively.

distance regimes, which decay on different length scales. We therefore show the short (green area) and long (gray area) distance regimes enlarged in Fig. S2 (b) and (c), respectively. Here, the two regimes are fitted separately with single exponential fits of the form $Ae^{d/\lambda_{\mathrm{m}}}$, where $A$ denotes the amplitude for zero distance. For the short (long) distance regime we determine the diffusion lengths to vary from $\lambda_{\mathrm{m}} \approx 1.0\,\mu\mathrm{m}$ to $0.8\,\mu\mathrm{m}$ ($\lambda_{\mathrm{m}} \approx 6.4\,\mu\mathrm{m}$ to $1.8\,\mu\mathrm{m}$) for magnetic fields from $\mu_0 H = 0.1\,\mathrm{T}$ to $7\,\mathrm{T}$. Since the long distances correspond to the diffusive regime [S3], we compare the diffusion lengths extracted for the long distances to the electrode separations studied in the main text and find that $\lambda_{\mathrm{m}} > d_{\mathrm{Pt}} = 1.6\,\mu\mathrm{m}$ for the whole field range considered. Hence, we conclude that the application of a spin-resistor model to our configuration is valid.

### C. Magnon conductivity as a function of magnetic field

As discussed in the main text, the magnon conductivity $\sigma_{\mathrm{m}}$ can be deduced from the spin-resistor model by the electrically excited transport of magnons between two known Pt electrodes (Pt2 and Pt1 in the main text). This was done as a function of magnetic field and is shown in Fig. S3. For small magnetic fields $10\,\mathrm{mT} < \mu_0 H < 50\,\mathrm{mT}$, the magnon conductivity in the YIG layer exhibits a sharp increase, which is due to the initial saturation of the magnetization. It reaches its maximum at $\sigma_{\mathrm{m}} \approx 3.2 \times 10^4\,\mathrm{S\,m^{-1}}$ for $\mu_0 H = 50\,\mathrm{mT}$,

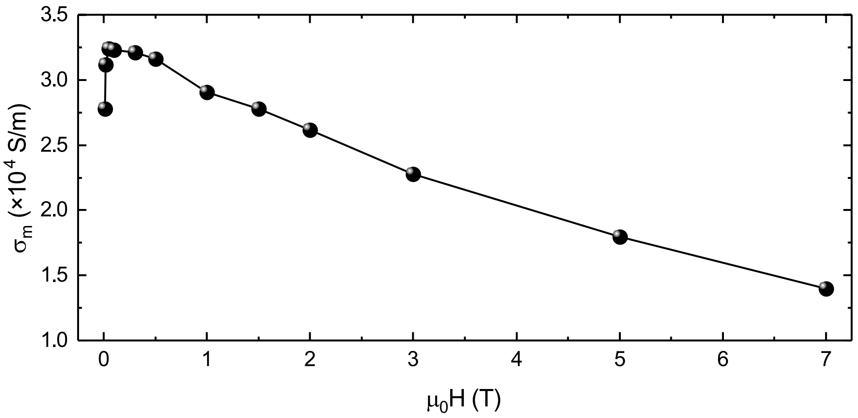


FIG. S3. Magnon conductivity $\sigma_{\mathrm{m}}$ of the YIG film as a function of magnetic field. The values were extracted within the spin-resistor model discussed in the main text.

which is roughly one order of magnitude smaller than what is reported in Ref. [S5]. This difference is due to the fact that our YIG film is five times thicker than the one studied in the previous work. Since the electrically excited magnon transport signal was shown to decrease monotonically with increasing thickness [S6], we conclude our extracted value to be reasonable. For larger magnetic fields $\mu_0 H > 50\,\mathrm{mT}$, $\sigma_{\mathrm{m}}$ monotonically decreases as a function of magnetic field. This is expected, since the thermal magnon number of the YIG film is decreasing as the Zeeman gap opens with increasing the external field. This is also reflected in the field dependence of the magnon diffusion length as discussed in the previous Section. In a Drude-inspired conductivity model for magnons [S7], a decreasing magnon number is directly connected to a decreasing magnon conductivity. We want to emphasize, that the extraction of $\sigma_{\mathrm{m}}$ as a function of magnetic field within the spin-resistor model implies, that we project the complete field dependence onto the magnon transport in YIG, which is paramaterized by the magnon conductivity. This, however, is justified since the spin conductance at the YIG/Pt interface (which is given by the spin mixing conductance, see Sec. A) is generally not considered as a field-dependent parameter [S2, S8]. Moreover, for the spin Hall angle of Pt no strong dependence on magnetic field was shown either [S4].

### D. Spin conductance $g_{\mathrm{CoFe}}$ and its effect on the anomalous spin Hall angle $\Theta_{\mathrm{ASH}}^{\mathrm{CoFe}}$

Having determined the field dependent magnon conductivity, the next step was to extract the spin conductance $g_{\mathrm{CoFe}}$ by modelling the absorption effect of the magnon current in

the CoFe electrode with the spin resistor-model (see main text). Substituting the magnon conductivities for each magnetic field into the spin-resistor network, we could calculate $g_{\mathrm{CoFe}}$ as a function of the spin diffusion length $\lambda_{\mathrm{CoFe}}$ by equating Eqs. (1) and (3a) from the main text. The result is shown in Fig. S4 (a) for different external magnetic fields. We here observe a vanishing dependence of $g_{\mathrm{CoFe}}$ on the spin diffusion length $\lambda_{\mathrm{CoFe}}$. As shown in the inset of Fig. S4 (a), the spin conductance only varies by roughly $\sim 0.05\,\%$ between $\lambda_{\mathrm{CoFe}} = 0\,\mathrm{nm}$ and 10 nm. We therefore treat $g_{\mathrm{CoFe}}$ as a constant value, independent of the spin diffusion length. However, as evident from Fig. S4 (a), the spin conductance does only slightly vary with the external magnetic field by a factor of $\sim 2$ in the measured field range. Similar to the YIG/Pt interface spin conductance $g_{\mathrm{Pt}}$, we do not expect the spin conductance $g_{\mathrm{CoFe}}$ at the YIG/CoFe interface to exhibit a strong external field dependence. Since our measurements of the detector voltage $V_{\mathrm{det}}(\mu_0 H)$ at the Pt3 electrode enter the spin-resistor model, this field dependence is projected onto $g_{\mathrm{CoFe}}$, as this parameter characterizes the amount of spin current absorbed in the CoFe strip (between Pt2 and Pt3). This effect is, however, mostly counterbalanced by the field dependent magnon conductivity values (see Fig. S3) that also enter the calculation of $g_{\mathrm{CoFe}}$. For the sake of consistency and to reduce the number of field dependent parameters, we therefore adopted a constant value of $g_{\mathrm{CoFe}} = 4 \times 10^{10}\,\mathrm{S\,m^{-1}}$ for the calculation of the anomalous spin Hall angle of CoFe in the main text. This value approximately corresponds to the values extracted for the field range between $\mu_0 H = 0.1\,\mathrm{T}$ and 2 T, as shown in Fig. S4 (a).

In order to show the effect of different spin conductances $g_{\mathrm{CoFe}}$ on the evolution of the anomalous spin Hall angle of CoFe, we plot $\Theta_{\mathrm{ASH}}^{\mathrm{CoFe}}$ as a function of magnetic field in Fig. S4 (b) for two constant values of $g_{\mathrm{CoFe}}$ (blue and orange points), assuming a constant spin diffusion length of $\lambda_{\mathrm{CoFe}} = 6\,\mathrm{nm}$ [S9]. Additionally we plot the situation when the full field dependence $g_{\mathrm{CoFe}}(\mu_0 H)$ shown in Fig. S4 (a) is taken into account (black data points). Assuming a small spin conductance $g_{\mathrm{CoFe}} = 2 \times 10^{10}\,\mathrm{S\,m^{-1}}$ (orange data), we find a significantly larger anomalous spin Hall angle as compared to $g_{\mathrm{CoFe}} = 4 \times 10^{10}\,\mathrm{S\,m^{-1}}$ (blue data). This is expected, since a smaller spin conductance has to be counterbalanced by a larger anomalous spin Hall angle, in order to maintain the measured magnon transport signal. Figuratetivly speaking, $g_{\mathrm{CoFe}}$ determines the amount of spin current injected into the CoFe strip, while $\Theta_{\mathrm{ASH}}^{\mathrm{CoFe}}$ describes the spin-to-charge current conversion process in the CoFe. Calculating $\Theta_{\mathrm{ASH}}^{\mathrm{CoFe}}$ including the full field dependence $g_{\mathrm{CoFe}}(\mu_0 H)$ (black data), we observe an increase

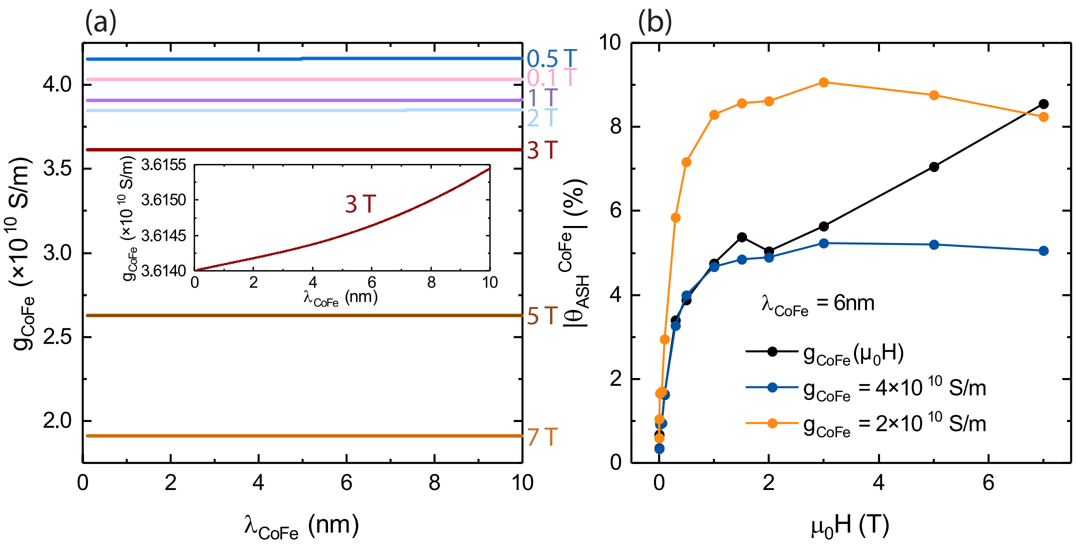


FIG. S4. (a) Spin conductance $g_{\mathrm{CoFe}}$ as a function of the spin diffusion length $\lambda_{\mathrm{CoFe}}$ for different external magnetic fields. The inset shows an enlarged view of one curve for $\mu_0 H = 3\,\mathrm{T}$. (b) Anomalous spin Hall angle of CoFe for two different (constant) values of the spin conductance $g_{\mathrm{CoFe}}$ (orange and blue datapoints). Additionally, the result for a field dependent spin conductance $g_{\mathrm{CoFe}}(\mu_0 H)$ is shown (black data points).

of the anomalous spin Hall angle even beyond 2 T, where the CoFe electrode is already saturated. This, however, is implausible and we thus conclude the assumption of a constant spin conductance $g_{\mathrm{CoFe}}$ to be justified.

### E. Asymmetry in magnon transport signals using spin injection/detection with CoFe electrodes

In the main text, we observed a slight asymmetry between the magnon transport signals measured at the CoFe detector for the two field directions pointing perpendicular to the strips, i.e. $\varphi = 0°$ and $\varphi = 180°$. Most likely, this asymmetry is related to the magnetization behaviour of $M_{\mathrm{CoFe}}$ of the CoFe electrode. We therefore measured the anisotropic magnetoresistance (AMR) as a function of $\varphi$ on the CoFe electrode in Fig. S5 (a). Additionally, we recorded the magnon transport signal as a function of $\varphi$ for various injector-detector configurations in Fig. S5 (b) - (e). Here, each of the respective panels is indicated with 'injector - detector', denoting the considered measurement configuration. For each configuration, we show rotations with two different magnetic field magnitudes (red and blue data

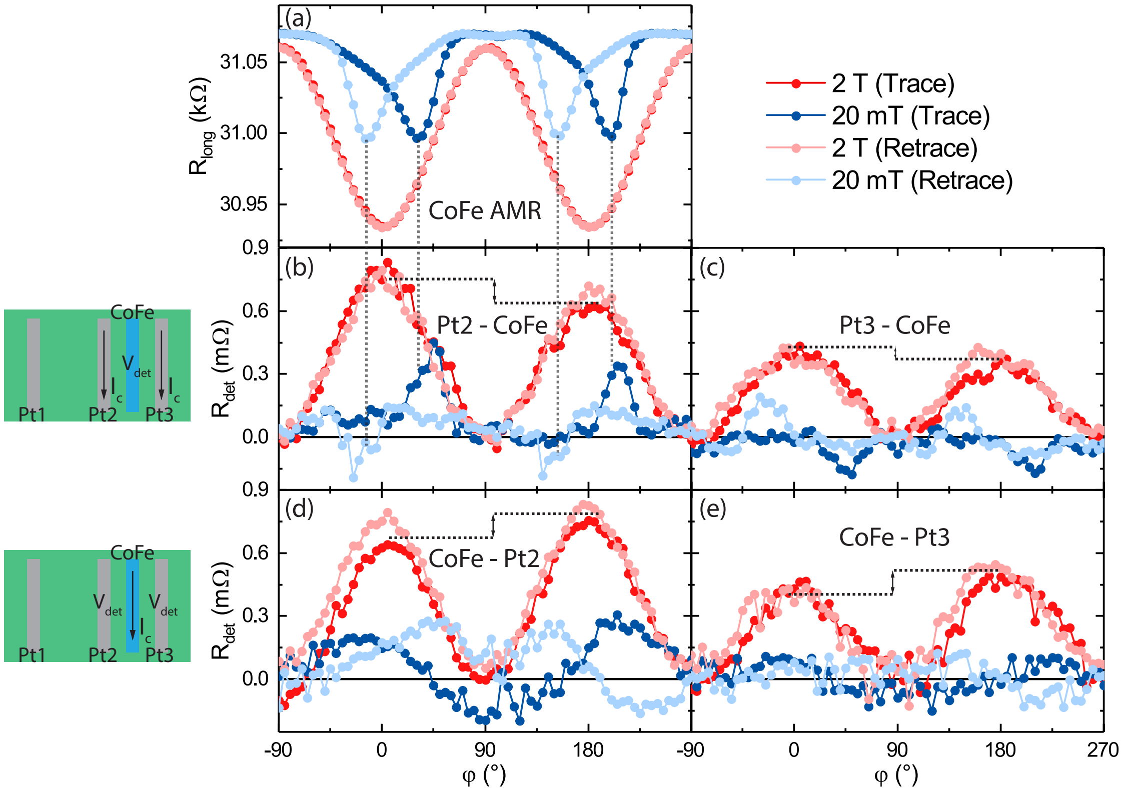


FIG. S5. (a) Longitudinal resistance $R_{\mathrm{long}}$ (i.e. the anisotropic magnetoresistance) of the CoFe electrode measured as a function of $\varphi$. Magnon transport signal $R_{\mathrm{det}}$ as a function of the magnetic field orientation $\varphi$. The forth (back) rotations of the magnetic field are shown in dark (light) colors. Different configurations of injector - detector combinations are used, which are indicated in the form of 'injector - detector' in each panel (b), (c), (d) and (e).

points), where the forth [towards larger positive $\varphi$ values] (back [towards smaller $\varphi$ values]) rotation is indicated by darker (lighter) colored points. Panels (b) and (c) show the case when the CoFe electrode is used as the detector, while panels (d) and (e) picture the case when the CoFe electrode serves as an injector.

We first focus on the high magnetic field ($\mu_0 H = 2\,\mathrm{T}$) rotations (red data points). Here, the AMR in CoFe (Fig. S5 (a)) exhibits the typical $\sin^2(\varphi)$ modulation with a relative magnitude of $\sim 3\,\%$, exhibiting a lower resistance state for a perpendicular configuration of $M_{\mathrm{CoFe}}$ as for a parallel alignment with the strip, i.e. the electrical current direction. Disregarding the asymmetry feature for now, the magnon transport signals in Fig. S5 (b) - (d) also show the expected behaviour (see main text). Nominally, we expect the signals of panel (b) and (c) to exhibit a comparable magnitude, since the injectors Pt2 and Pt3

are supposed to have the same edge-to-edge distance of $d = 300\,\mathrm{nm}$ to the CoFe electrode. In contrast to this, the signal amplitudes differ by roughly 45 %. Considering the distance dependence of the magnon transport in the YIG film (Fig. S2), we see that the transport signal varies by roughly 25 % from $d = 300\,\mathrm{nm}$ to $d = 200\,\mathrm{nm}$. Hence, this difference can be explained by a slight displacement of the CoFe strip by $\sim 80\,\mathrm{nm}$ in the negative $y$ direction (see Fig. 1 in the main text), which is likely due to an error in the alignment procedure during the fabrication of the samples. When we calculate the anomalous spin Hall angle with our spin-resistor model and include this displacement to the model, it only changes the value of $\Theta_{\mathrm{ASH}}^{\mathrm{CoFe}}$ by  0.5 %. The lower panels (d) and (e) present the signals at the Pt2 and Pt3 electrode, when the CoFe strip is used as the injector. Here, the difference in signal magnitude can be again attributed to the displacement of the CoFe electrode in the same quantitative way, thus supporting this claim.

A more interesting behaviour is observed for the small magnetic field ($\mu_0 H = 20\,\mathrm{mT}$) rotations (blue data points). Here, the AMR in CoFe (Fig. S5 (a)) exhibits a clear hysteresis due to the shape anisotropy of the electrode: the resistance switches for $\varphi > 0°$ ($\varphi > 180°$) for the forth rotation (dark blue), rather than directly at $\varphi = 0°$ ($\varphi = 180°$). As expected, this behaviour is inverted for the back rotation (light blue), showing a switching for $\varphi < 180°$ ($\varphi < 0°$). The magnon transport signal measured for the 'Pt2 - CoFe' configuration (Fig. S5 (b)) exhibits several peaks in the signal modulation, which approximately correspond to the magnetization switching of $M_{\mathrm{CoFe}}$ to a perpendicular state (indicated by the gray dashed vertical lines). These peaks are attributed to the increase of the magnon transport signal when the magnetization $M_{\mathrm{CoFe}}$ has a finite contribution perpendicular to the strip, such that the anomalous spin Hall effect (ASHE) becomes measurable along the strip. Unexpectedly, the back rotation exhibits these peaks with an inverted sign. This is most likely due to an opposing configuration of the YIG magnetization $M_{\mathrm{YIG}}$ and $M_{\mathrm{CoFe}}$ at these inverted peaks. Since the spin current polarization due to the ASHE is tunable via the magnetization direction of $M_{\mathrm{CoFe}}$, and the diffusion direction of the Pt-injected magnons is determined by $M_{\mathrm{YIG}}$, the sign of the resulting signal in the CoFe detector is dependent on the relative orientation of the two magnetizations. At the considered field of $\mu_0 H = 20\,\mathrm{mT}$, $M_{\mathrm{YIG}}$ can be assumed to closely follow the external magnetic field direction. $M_{\mathrm{CoFe}}$, however, is pinned due to the shape anisotropy of the strip. Thus, the inverted peaks in the back rotation in Fig. S5 (b) might be attributed to a rather complicated domain configuration

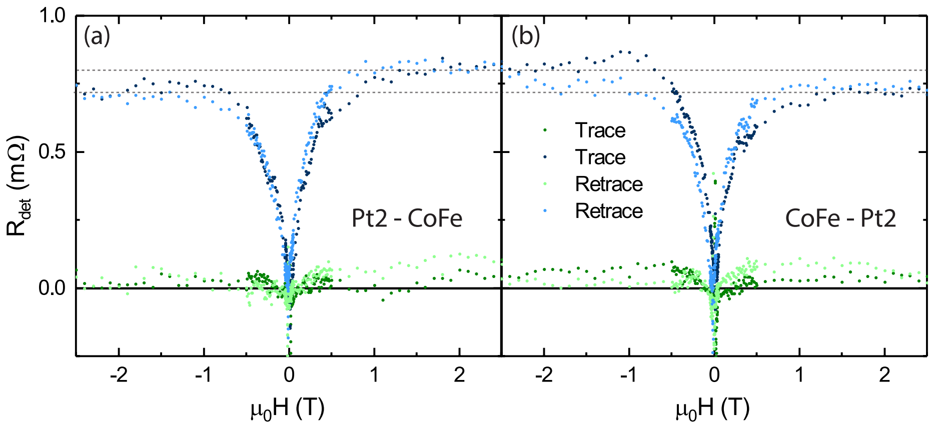


FIG. S6. Measurements as a function of magnetic field strength for field directions pointing perpendicular (blue) and parallel (green) to the strip length. Dark and light colored lines correspond to trace and retrace curves, respectively. In (a) the magnon transport signal for the Pt2 - CoFe (injector - detector) configuration is shown, which is inverted in (b).

in the CoFe electrode during the rotation, which can exhibit a net contribution of $M_{\mathrm{CoFe}}$ pointing oppositely to $M_{\mathrm{YIG}}$. Here, it is important to note that in our experiments we conducted rotations over 400° in each direction and thus a slight misalignment with respect to the structure could be responsible for a different domain configuration for the two rotation directions. A similar peak structure can be observed for the 'Pt2 - CoFe' configuration in Fig. S5 (c). Strangely, however, the peaks are exactly inverted regarding the forth and back rotations, as compared to the behaviour for 'Pt2 - CoFe' configuration in Fig. S5 (b). Since the two measurements in panel (b) and (c) are obviously not measured in the same run, one could argue that the system was prepared differently regarding its domain configuration, resulting in a different relative orientation of $M_{\mathrm{CoFe}}$ and $M_{\mathrm{YIG}}$ during the rotation. The small magnetic field rotations for the case when the CoFe electrode is used as the injector, shown in Fig. S5 (d) and (e), do however not exhibit a clear modulation of the signal. All in all, the observed behaviour at small magnetic field rotations supports the picture that the shape anisotropy in the CoFe strip is the origin of the oberved features. Moreover, it supports the claim that the anomalous spin Hall angle in CoFe is responsible for the observed magnon transport signals, since the peak structure in the rotations suggests a very sensitive dependence on the relative orientation of $M_{\mathrm{CoFe}}$ with respect to $M_{\mathrm{YIG}}$.

In the following, we focus on the asymmetry behaviour for $\mu_0 H = 2\,\mathrm{T}$ in Fig. S5 (b) - (e) (red data points). Interestingely, the asymmetry feature for panel (b) and (c) (CoFe as detector) exhibits an inverted behaviour as compared to the lower panels (d) and (e) (CoFe as injector), suggesting that the asymmetry is reversed when the CoFe electrode is either used as an injector or detector. In order to further solidify the appearance of this feature, we plot the fieldsweep measurements for the 'Pt2 - CoFe' and 'Pt2 - CoFe' configurations in Fig. S6 (a) and (b), respectively. As evident, we still oberve the asymmetry for magnetic fields $\mu_0 H \gtrsim 2\,\mathrm{T}$ and confirm the inversion of the feature when the CoFe electrode is changed from being used as a detector or injector (indicated by the horizontal gray dashed lines). Several possible sources of the observed asymmetry feature can be thought of in our device. The fact, that the asymmetry is larger for high magnetic fields rules out any effects stemming from a misalignment of the YIG and CoFe magnetizations. Apart from this, the asymmetry behaviour does also not depend on the actual direction of the magnon spin current (i.e. magnon current flowing to the left or right from the CoFe injector, as measured in Fig. S5 (d) and (e)), therefore ruling out any anisotropic magnon mode propagation effects. As theoretically proposed in Ref. [S10], the observed asymmetry effect does resemble an unidirectional magnon transport effect. Here, the asymmetry is stemming from a non-linear injection of magnons but a linear depletion of the magnon system as a function of the injector current. Since our orientation dependent measurements switch between injection and depletion of the magnon system by reversing the magnetic field direction, an imbalance of the signal amplitudes similar to our results could occur. However, our current reversal method that we use for the detection of the electrically excited magnons is not sensitive to any current-induced imbalance between injection and depletion of magnons, hence ruling out non-linear magnon injection effects as well. For the same reason, we cannot attribute any effects arising from the difference in the density of states of the majority and minority spins in the ferromagnetic CoFe electrode. Due to the ASHE, the amount of electron spins on the top and bottom side of the CoFe electrode are not equal, hence one could relate the asymmetry to an asymmetric spin injection for different field directions. On the one hand, however, the current reversal method averages out this putative imbalance. On the other hand, it is not the actual amount of spins at particularly the YIG/CoFe interface that determines the spin injection but rather the spin chemical potential, which is equal for both field directions [S1, S3]. In conclusion, the asymmetry behaviour of

magnon injection/detection with CoFe electrodes appears to be robust in our measurements. It is, however, not yet clear which mechanism is responsible for this interesting feature and requires further investigation.

### F. Shape anisotropy of the CoFe electrode

In this Section, we employ the Stoner-Wohlfarth model [S11] to extract the uniaxial shape anisotropy of the CoFe electrode. On the basis of this model, we furthermore try to reproduce the field dependence of the anomalous spin Hall angle $\Theta_{\mathrm{ASH}}^{\mathrm{CoFe}}$, which is characterized by the aligning of the magnetization $M_{\mathrm{CoFe}}$ perpendicular to the CoFe strip (i.e. along the magnetic hard axis). The Stoner-Wohlfarth model with uniaxial shape anisotropy (for our definition of the field direction) reads

$$f = -\frac{1}{2}K_{\mathrm{u}}\sin^2(\theta+\varphi) - \mu_0 H M_{\mathrm{CoFe}}\cos(\theta), \tag{S2}$$

where $f$ is the free energy density, $K_{\mathrm{u}}$ is the uniaxial anisotropy constant, $\mu_0 H$ the external magnetic field strength with $\mu_0$ the magnetic vacuum permeability, $\mu_0 M_{\mathrm{CoFe}} \approx 2.3\,\mathrm{T}$ is the saturation magnetization of CoFe [S12], $\varphi$ is the direction of the external magnetic field with respect to the magnetic hard axis and $\theta$ is the angle between the magnetization and external field direction. Equation (S2) is expanded up to second order in $\theta$ and then minimized with respect to $\theta$. The resulting equation for $\theta$ is a function of the angle $\varphi$ and reads

$$\theta(\varphi) = \frac{K_{\mathrm{u}}\cos(\varphi)\sin(\varphi)}{\mu_0 H M_{\mathrm{CoFe}} - K_{\mathrm{u}}\cos(2\varphi)}. \tag{S3}$$

The AMR modulates as a $\sin^2(\varphi)$ function when the magnetization is rotated in the magnetic material. Introducing the finite misalignment of the external magnetic field and the magnetization, the AMR modulation can be written as $\sin^2(\varphi-\theta(\varphi))$ with Eq. (S3). This function is fitted to the AMR measurements of the CoFe electrode for different magnetic fields in Fig. S7 (a). Extracting the anisotropy constant from the fits gives roughly $K_{\mathrm{u}} = 90\,\mathrm{kJ\,m^{-3}}$, which gives an equivalent anisotropy field of $B_{\mathrm{ani}} = K_{\mathrm{u}}/M_{\mathrm{CoFe}} \approx 49\,\mathrm{mT}$.

Using the experimentally extracted anisotropy constant $K_{\mathrm{u}}$, we can calculate the field dependence of the anomalous spin Hall angle $\Theta_{\mathrm{ASH}}^{\mathrm{CoFe}}$ shown in Fig. S7 (b). For the purpose of this, Eq. (S2) is minimized with respect to the angle $\theta$ while setting $\varphi = 0°$ (which corresponds to the magnetic hard axis of the field direction). Eventually, we extract the angle

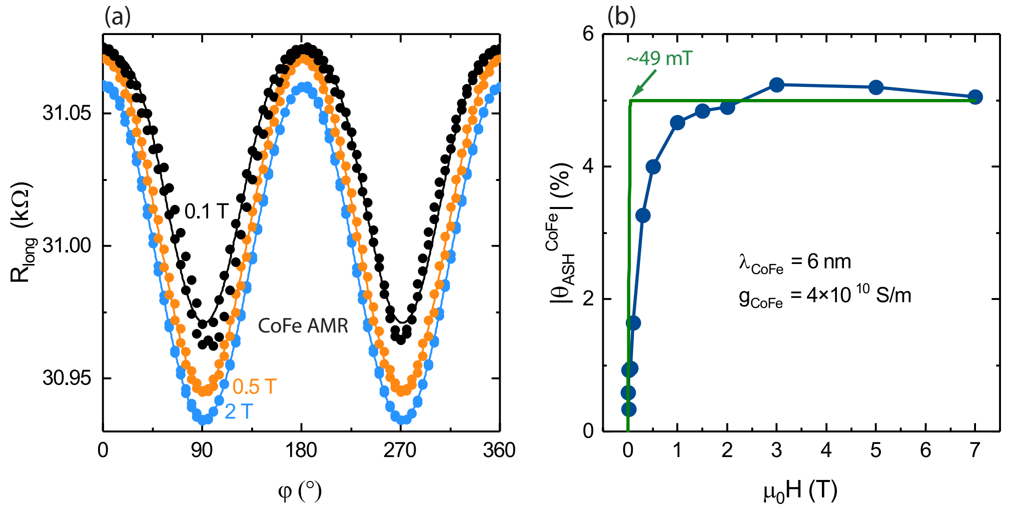


FIG. S7. (a) Longitudinal resistance $R_{\mathrm{long}}$ measured at the CoFe electrode as a function of the magnetic field orientation $\varphi$, showing the anisotropic magnetoresistance behaviour. The solid lines are fits to the data. (b) Field dependence of the anomalous spin Hall angle $\Theta_{\mathrm{ASH}}^{\mathrm{CoFe}}$ (same as Fig. 4 (d) of the main text). The green solid line is calculated on the basis of a Stoner-Wohlfarth model assuming uniaxial shape ansisotropy of the CoFe strip with an anisotropy field $B_{\mathrm{ani}} \approx 49\,\mathrm{mT}$.

$\theta_{\mathrm{min}}$ as a function of the external magnetic field $\mu_0 H$. Taking into account the measured spin Hall angle at large magnetic fields ($\sim 5\,\%$) and considering the projection of the magnetization along the magnetic hard axis (i.e. $\cos(\theta_{\mathrm{min}})$), we expect a field dependence as shown by the green line in Fig. S7 (d). As evident, this simple model does not reproduce the observed field dependence well, concluding that the CoFe electrode is in a multidomain state for small magnetic fields $\mu_0 H \lesssim 1\,\mathrm{T}$.

---


[S1] Y.-T. Chen, S. Takahashi, H. Nakayama, M. Althammer, S. T. B. Goennenwein, E. Saitoh, and G. E. W. Bauer, Physical Review B **87**, 144411 (2013).

[S2] A. Brataas, Y. V. Nazarov, and G. E. W. Bauer, Physical Review Letters **84**, 2481 (2000).

[S3] L. J. Cornelissen, K. J. H. Peters, G. E. W. Bauer, R. A. Duine, and B. J. van Wees, Physical Review B **94**, 014412 (2016).

[S4] M. Althammer, S. Meyer, H. Nakayama, M. Schreier, S. Altmannshofer, M. Weiler, H. Huebl, S. Geprägs, M. Opel, R. Gross, D. Meier, C. Klewe, T. Kuschel, J.-M. Schmal-

horst, G. Reiss, L. Shen, A. Gupta, Y.-T. Chen, G. E. W. Bauer, E. Saitoh, and S. T. B. Goennenwein, Physical Review B **87**, 224401 (2013).

[S5] L. J. Cornelissen, J. Shan, and B. J. van Wees, Physical Review B **94** (2016), 10.1103/physrevb.94.180402.

[S6] J. Shan, L. J. Cornelissen, N. Vlietstra, J. B. Youssef, T. Kuschel, R. A. Duine, and B. J. van Wees, Physical Review B **94** (2016), 10.1103/physrevb.94.174437.

[S7] L. J. Cornelissen, J. Liu, B. J. van Wees, and R. A. Duine, Physical Review Letters **120**, 097702 (2018).

[S8] M. Weiler, M. Althammer, M. Schreier, J. Lotze, M. Pernpeintner, S. Meyer, H. Huebl, R. Gross, A. Kamra, J. Xiao, Y.-T. Chen, H. Jiao, G. E. W. Bauer, and S. T. B. Goennenwein, Physical Review Letters **111**, 176601 (2013).

[S9] G. Zahnd, L. Vila, V. T. Pham, M. Cosset-Cheneau, W. Lim, A. Brenac, P. Laczkowski, A. Marty, and J. P. Attané, Physical Review B **98** (2018), 10.1103/physrevb.98.174414.

[S10] X.-g. Wang, Z.-w. Zhou, Y.-z. Nie, Q.-l. Xia, and G.-h. Guo, Physical Review B **97**, 094401 (2018).

[S11] E. C. Stoner and E. P. Wohlfarth, Philosophical Transactions of the Royal Society A: Mathematical, Physical and Engineering Sciences **240**, 599 (1948).

[S12] M. A. W. Schoen, D. Thonig, M. L. Schneider, T. J. Silva, H. T. Nembach, O. Eriksson, O. Karis, and J. M. Shaw, Nature Physics **12**, 839 (2016).
